# Supplementary material for: Lineage-Aware Temporal Windows: Supporting Set Operations in Temporal-Probabilistic Databases
Source: arXiv:1910.00474 source file (2019-10-01)
Supplement: Supplementary file 1 [file 9_appendix.tex]

%----------------------------------------------------------------------------------------
%	Appendix
%----------------------------------------------------------------------------------------
\section*{APPENDIX}

\begin{tikzpicture}
%\begin{loglogaxis}[
\begin{axis}[
xlabel={Degrees of freedom},
ylabel={$L_2$ Error}
xtick={20, 40, 60, 80, 100, 120, 140, 160, 180, 200},
xmin=20,
xmax=200,
ymax=200000
]
% NORM
\addplot coordinates {
(20 ,65978.87)
(40 ,263905.97)
(60 ,591278.94)
(80 ,1054493.6)
(100,1648709.9)
(120,2374035.2)
(140,3262059.8)
(160,4210019)
(180,5318095)
(200,6599149.5)};

%OIP
\addplot coordinates{
(20 ,7.2045994)
(40 ,15.9494)
(60 ,26.801199)
(80 ,37.723)
(100,64.2594)
(120,63.7962)
(140,77.367)
(160,94.4076)
(180,110.690605)
(200,121.6188)
};

%SWA
\addplot coordinates{
(20 ,16.145819)
(40 ,31.84674)
(60 ,49.971043)
(80 ,63.551903)
(100,86.30694)
(120,92.7451)
(140,116.487)
(160,140.24341)
(180,149.0686)
(200,164.9032)
};

%TI
\addplot coordinates{
(20 ,3251.6045)
(40 ,13146.192)
(60 ,29592.7)
(80 ,52745.89)
(100,82532.89)
(120,118979.36)
(140,161329.25)
(160,210760.48)
(180,266898.2)
(200,330802.97)
};

%TPE
\addplot coordinates{
(20 ,1327.6)
(40 ,3486.2)
(60 ,6625.8)
(80 ,10752.8)
(100,16005.6)
(120,21787)
(140,29412.8)
(160,37167.8)
(180,46508)
(200,55503)};
\legend{NORM,OIP,SWA,TI,TPE}
%\end{loglogaxis}
\end{axis}
\end{tikzpicture}

\subsection{Precise Size of LIR}

In order to compute the precise number of tuples included in the
result of the {\bf LIR}, we determine the redundant cases included
in the definition of the upper bound. The upper bound considers all
the start/end points in tuples of ${\bf r}$ or ${\bf s}$ as
potential start-points of an interval in a tuple of the {\bf LIR}.
Consequently, it counts up  $[T_s,T_e)$ intervals during which no tuple
in ${\bf r}$ or ${\bf s}$ is valid. Such an interval could be
$[09,10)$ in Fig.~\ref{fig:upperBound}. Moreover, when a time-point
exists both in ${\bf r}$ and ${\bf s}$, such as time-points $1$
and $9$ in Fig.~\ref{fig:upperBound}, it will be a start-point only
for one output tuple. However, it's counted as two different
start-points in the upper bound.

\begin{proposition}
\label{prop:LIRsizePrecise}
Let ${\bf r}$,${\bf s}$ be temporal probabilistic relations with schema
$(F, T,\lambda)$. The size of result of $LIR({\bf r};{\bf s})$
is equal to: 

\begin{equation}
|LIR({\bf r};{\bf s})| = |SE_{R} \cup SE_{S}| - |EI_{SR}| -1
\end{equation} 
 
where $SE_{R}$, $SE_{S}$ are sets including all the start/end points of the tuples,
respectively and $EI_{SR}$ is the set of valid intervals $[t_s$,$t_e)$, with $t_s,
t_e\in SE_{R} \cup SE_{S}$, where no tuple from ${\bf r}$ or ${\bf s}$ is
valid. 
%$EI_{SR}=\{[t_s,t_e)|t_s,t_e\in (SE_{R} \cup SE_{S}) \wedge t_s>t_e
%\wedge \forall r\in {\bf r}(r.T \cap [t_s,t_e) \neq \emptyset)
%\wedge \forall s\in {\bf s}(s.T \cap [t_s,t_e) \neq \emptyset) \}$.
\end{proposition}

The computation of $|SE_{R} \cup SE_{S}|$ instead of the sum of
start/end points guarantees that time-points in intervals of the tuples
of both $S_R$ and $S_S$ are not counted twice. 
In Fig.~\ref{fig:upperBound}, below the axis are the tuples in the
result of {\bf LIR}. No-attention is given to their lineage
expressions or exact intervals. The number of tuples in the LIR
result is 9 since $|SE_{R1}\cup SE_{S1}|=10$, $|EI_{SR}|=1$.

\subsection{Lemmas}

\begin{lemma}
\label{lem:mainObservation}
Assume two temporal probabilistic relations ${\bf r}$ and ${\bf s}$
with schema $(F, T, \lambda)$ and  the set of the base tuples $L_{b}(\lambda)$
in lineage expression $\lambda$. All the facts included in ${\bf r}\cap^\kat{TP}
{\bf s}$ or ${\bf r}-^\kat{TP}{\bf s}$ are included, during the same
intervals, in the result of ${\bf r}\cup^\kat{TP}{\bf s}$.

\vspace*{0.1cm}
% {\centering \noindent $\exists k \in {\bf k} \ (k.F=f \ \wedge
% \ k.T = T_\kat{F} \ \wedge \ \lambda_\kat{F} = \lambda_{fun}(\lambda_1,\lambda_2))$}
$\pi_{F,T,L_{b}(\lambda)}({\bf r}\cup^\kat{TP}{\bf s}) \supseteq
 \pi_{F,T,L_{b}(\lambda)}({\bf r}-^\kat{TP}{\bf s}) \supseteq
 \pi_{F,T,L_{b}(\lambda)}({\bf r}\cap^\kat{TP}{\bf s})$
\end{lemma}

\vspace*{0.1cm}
\begin{proof}
All the inclusion relationships in Lemma~\ref{lem:mainObservation} can be
similarly proven and thus,  we will only prove $\pi_{F,T,L_{b}
(\lambda)}({\bf r}\cup^\kat{TP}{\bf s}) \supseteq \pi_{F,T,L_{b}(\lambda)}
({\bf r}\cap^\kat{TP}{\bf s})$. For this inclusion to hold, all tuples 
belonging in
$\pi_{F,T,L_{b}(\lambda)}({\bf r}\cap^\kat{TP}{\bf s})$ should also belong to
$\pi_{F,T,L_{b}(\lambda)}({\bf r}\cup^\kat{TP}{\bf s})$. We will assume
that the statement $\exists u \in \pi_{F,T,L_{b}(\lambda)}({\bf r}\cap^\kat{TP}
{\bf s})\ (u \notin \pi_{F,T,L_{b}(\lambda)}({\bf r}\cup^\kat{TP}{\bf s}))$
(1) and show that this assumption leads to contradiction.

%Relations $\pi_{F,T,L_{b}(\lambda)/\lambda_{set}}({\bf r}\cup^\kat{TP}
%{\bf s})$ and $\pi_{F,T,L_{b}(\lambda)/\lambda_{set}}({\bf r}\cap^
%\kat{TP}{\bf s})$ include all the tuples in ${\bf r}\cup^\kat{TP}{\bf s}$
%and ${\bf r}\cup^\kat{TP}{\bf s}$, after their lineage expressions have been
%replaced by the corresponding set of base tuples $L_b(\lambda)$. Consequently,
%each tuple in these relations

Assume tuple $u \in \pi_{F,T,L_{b}(\lambda)/\lambda_{set}}({\bf r}\cap^
\kat{TP}{\bf s})$. As all tuples in this relation, $u$ has been derived from
a tuple $u' \in \ {\bf r}\cap^\kat{TP}{\bf s}$ with $u'.F = u.F \wedge
u'.T = u.T \wedge L_{b}(u'.\lambda) = u.\lambda_{set}$. Given that $u$ and $u'$
include the same fact and interval, it holds that $r_u = r_{u'} \wedge s_u = s_{u'}$.
Moreover, since $u'$ belongs to the result of the TP set intersection, according
to Definition~\ref{def:TPsetOps}, it satisfies the corresponding interval condition
$i_c(u')$, the fact condition $r_{u'} \ne \mathtt{null} \wedge s_{u'} \ne \mathtt{null}$ and the
lineage condition $u.\lambda = r_{u'}.\lambda \cdot s_{u'}.\lambda$. Consequently,
$u$ also satisfies the above interval and fact conditions. Also, by ignoring the
logical operators, the set of base tuples included in $u.\lambda_{set}$ is equal to
$L_{b}(u'.\lambda) = L_{b}(r_{u'}.\lambda \cdot s_{u'}.\lambda) = L_b(r_{u}.\lambda))
\cup L_b(s_{u}.\lambda)$. 

According to our initial assumption (1), $u \notin \pi_{F,T,L_{b}(\lambda)/
\lambda_{set}}({\bf r}\cup^\kat{TP}{\bf s})$. This means that $u$ cannot
have been derived from any tuple in ${\bf r}\cup^\kat{TP}{\bf s}$. So,
for all tuples $u''$ over the schema (F,T,$\lambda$,p) with $u'.F = u.F \wedge
u'.T = u.T \wedge L_{b}(u''.\lambda) = u.\lambda_{set}$, we conclude that $u''
\notin {\bf r}\cup^\kat{TP}{\bf s}$. Given that $u$ and $u'$ include the
same fact and interval, it holds that $r_u = r_{u''} \wedge s_u = s_{u''}$.  
Also, given the interval and fact condition satisfied by $u$, it holds that $u''$
satisfies $i_c(u'')$ and $r_{u''} \ne \mathtt{null} \wedge s_{u''} \ne \mathtt{null}$. However,
$u''\notin {\bf r}\cup^\kat{TP}{\bf s}$. For this to hold, based on
Table~\ref{def:TPsetOps} and the interval and fact conditions that $u''$ satisfies,
$u''.\lambda \neq r_{u''}.\lambda \cdot s_{u''}.\lambda$. As a consequence
$L_{b}(u''.\lambda) \neq L_b(r_{u''}.\lambda)) \cup L_b(s_{u''}.\lambda) \neq
L_b(r_{u}.\lambda)) \cup L_b(s_{u}.\lambda)$. This contradicts our assumption
that $L_{b}(u''.\lambda) = u.\lambda_{set}$ prooving that $u \notin \pi_{F,T,L_{b}
(\lambda)/\lambda_{set}} ({\bf r}\cup^\kat{TP}{\bf s})$ is false, and thus
$\pi_{F,T,L_{b} (\lambda)}({\bf r}\cup^\kat{TP}{\bf s}) \supseteq
\pi_{F,T,L_{b}(\lambda)} ({\bf r}\cap^\kat{TP}{\bf s})$.
\end{proof}

%Also,
%$L_{b}(u'.\lambda) = L_{b}(r_{u}.\lambda
%\cdot s_{u}.\lambda) = L_b(r_{u}.\lambda)) \cup L_b(s_{u}.\lambda) = L_{b}
%(r_{u}.\lambda + s_{u}.\lambda)$. Consequently, it could have been derived by
%a tuple $u''$ in ${\bf r}\cup^\kat{TP}{\bf s}$ with $u''.F = u.F \wedge
%u''.T = u.T$ (and thus $r_u = r_{u''} \wedge s_u = s_{u''}$) satisfying the
%interval condition, the same fact condition as $u$ and having lineage expression
%$u''.\lambda = r_{u''}.\lambda + s_{u''}.\lambda$. The existence of such a tuple
%contradicts our assumption of 
In Lemma~\ref{lem:mainObservation}, the projections remove the probability
attribute and transform the lineage from a boolean expression to a set. For example,
$\pi_{F,T,L_{b}(\lambda)} ({\bf r}\cap^\kat{TP}{\bf s})$ includes
the tuples \textit{(m,  [2,4), \{$r_1$,$s_1$\})}, \textit{(m,  [6,8), \{$r_1$,
$s_2$\})} and \textit{(c,  [4,5), \{$r_2$,$s_3$\})}. Given this transformation,
the inclusion relations in Lemma~\ref{lem:mainObservation} indicate that there is
an overlap on the information included in the result of all TP set operations. 
The overlaps relates to facts that are included in at least one of the input relations
and, during a time interval, the lineages of the input tuples are differently
combined to form a final lineage expression, depending on the operation applied.
For example, given the relations ${\bf r}$ and ${\bf s}$ (fig.~\ref{fig:tpdbEx})
the fact \textit{(m,b)} during the interval $[2,4)$ is relevant for all TP operations
applied on ${\bf r}$ and ${\bf s}$. However, its lineage expression varies
based on the operation: in TP set difference it is $r_1 \cdot ! s_1$
(Fig.~\ref{fig:tpdbResult}, in TP set union it is $r_1 + s_1$ and in TP set
intersection it $r_1 \cdot s_1$ (Figure \ref{fig:tpSetOps}).

However, there are also time intervals during which, facts included in one of the input
relations are not relevant for the result of all temporal probabilistic set operations.
For example, given the relations ${\bf r}$ and ${\bf s}$ (Fig.~\ref{fig:tpdbEx}),
the tuple \textit{(c,b,[7,9), \{$s_3$\})} is only included in $\pi_{F,T,L_{b} (\lambda)}
({\bf r}\cup^\kat{TP}{\bf s})$. Thus, the fact \textit{(c,b)} during the interval
\textit{[7,9)}, included in a tuple of relation ${\bf s}$, is only relevant for the
TP set union leading to the output tuple \emph{(m,  [7,9), $s_3$, 0.7)}.

\begin{lemma}
\label{lem:secondObservation}
Assume two temporal probabilistic relations ${\bf r}$ and ${\bf s}$ with
schema $(F, T, \lambda)$ and the set of the base tuples $L_{b}(\lambda)$
in lineage expression $\lambda$. All the facts included in tuples of $LIR
({\bf r},{\bf s})$ are also included, during the same intervals, in
tuples of ${\bf r} \cup {\bf s}$ and vice versa.

\vspace*{0.2cm}
% {\centering \noindent $\exists k \in {\bf k} \ (k.F=f \ \wedge
% \ k.T = T_\kat{F} \ \wedge \ \lambda_\kat{F} = \lambda_{fun}(\lambda_1,\lambda_2))$}
\centering{$\pi_{F,T,L_{b}(\mathtt{\lambda_r}) \cup L_{b}(\mathtt{\lambda_s})  }(LIR({\bf r},{\bf s}))
\equiv \pi_{F,T,L_{b}(\lambda)}({\bf r}\cup^\kat{TP}{\bf s})$}
\end{lemma}

%Given two relations ${\bf r}$ and ${\bf s}$, the LIR computes, each fact
%$f$ included in any of the two relations at any time-point $t$ as well as the
%lineage expressions of the tuples in ${\bf r}$ and ${\bf s}$, including
%$f$. Equivalently, the TP set union of ${\bf r}$ and ${\bf s}$ includes
%the facts for which there is a probability to be in ${\bf r}$ or in ${\bf s}$.
The proof of Lemma~\ref{lem:secondObservation} is similar to the proof of
Lemma~\ref{lem:mainObservation} and thus, due to space limitations can be 
found in the Appendix. Based on Lemma~\ref{lem:secondObservation}, {\bf LIR}
contains the same information with the result of TP set union. This can also be observed
by comparing $LIR({\bf r},{\bf s})$ (Fig.~\ref{tab:tpdbLIR}) and
$({\bf r} \cup^\kat{TP} {\bf s})$ (Fig.~\ref{tab:unRS}) of relations
${\bf r}$ and ${\bf s}$ of Fig.~\ref{fig:tpdbEx}). Foe example, tuple
\textit{(m,  [2,4), \{$r_1 + s_1$\})} is included in the TP set union and
tuple \textit{(m,  [2,4), $r_1$, $s_1$)} is included in the temporal
bi-lineage relation produced by {\bf LIR}.

%included in $LIR({\bf r},{\bf s})$. Similarly, the same tuple is included in $\pi_{F,T,L_{b}(\mathtt{\lambda_r})
%\cup L_{b}(\mathtt{\lambda_s})}(LIR({\bf r},{\bf s}))$ since tuple \textit{(m, 
%[2,4), $r_1$, $s_1$)} 
%and $L_{b}(\mathtt{\lambda_r})$ $\cup$ $L_{b}(\mathtt{\lambda_s})$ $=$ $\{r_1,s_1\}$.

\subsection{Detailed Execution of the ELIR}
\label{sec:ELIRdetailed} 

%%%%%%%%%%%%%%%%%%%%%%%%%%%%%%% EXAMPLE %%%%%%%%%%%%%%%%%%%%%%%%%%%%%%%%%%%%%%% 
 \begin{center}
 \begin{table}[ht]
 \center
 \scalebox{0.8}{
 \begin{tabular}{ | c !{\VRule[1.5pt]} c| c| c| c| c| c |c |c|}
 \multicolumn{8}{l}{}\\ \hline
                  i  & {\bf sG} & {\bf gRep} & {\bf upc}   & {\bf rT} & {\bf sT} & {\bf sP} 
                     & {\bf bP} & {\bf out}\\ \specialrule{1.2pt}{0pt}{0pt}
 \multirow{5}{*}{1}  & TRUE & $x_1$ & $x_1$ & -     & $x_1$ & 1 & 1  & - \\ \cline{2-9}
                     & TRUE & $x_1$ & $x_2$ & -     & $x_1$ & 1 & 2  & (m,b,[1,2),-,$s_1$) \\ \cline{2-9}
                     & TRUE & $x_1$ & -     & $x_2$ & $x_1$ & 2 & 2  & - \\ \cline{2-9}
                     & TRUE & $x_1$ & -     & $x_2$ & $x_1$ & 2 & 4  & - \\ \cline{2-9}
                     & TRUE & $x_1$ & -     & $x_2$ & -     & 4 & 4  & (m,b,[2,4),$r_1$,$s_1$)\\ \specialrule{1.2pt}{0pt}{0pt}
 
 \multirow{2}{*}{2}  & TRUE & $x_1$ & $x_3$ & $x_2$ & - & 4 & 6 & - \\ \cline{2-9}
                     & TRUE & $x_1$ & $x_3$ & $x_2$ & - & 6 & 6 & (m,b,[4,6),$r_1$,-)\\ \specialrule{1.2pt}{0pt}{0pt}
 
 \multirow{2}{*}{3}  & TRUE & $x_1$ & - & $x_2$ & $x_3$ & 6 & 8 & - \\ \cline{2-9}
                     & TRUE & $x_1$ & - & $x_2$ & -     & 8 & 8 & (m,b,[6,8),$r_1$,$s_2$)\\ \specialrule{1.2pt}{0pt}{0pt}
 
 \multirow{2}{*}{4}  & FALSE & $x_1$  & $x_4$ & $x_2$ &   -   & 8 & 10 & -\\ \cline{2-9}
                     & TRUE  & $x_4$  & -     & -     & $x_4$ & 4 & 4 & (m,b,[8,10),$r_1$,-)\\  \specialrule{1.2pt}{0pt}{0pt}

 \multirow{2}{*}{5}  & TRUE & $x_4$ & - & $x_5$ & $x_4$ & 4 & 5 & - \\ \cline{2-9}
                     & TRUE & $x_4$ & - & -     & -     & 5 & 5 & (c,b,[4,5),$r_2$,$s_3$)\\ \specialrule{1.2pt}{0pt}{0pt}
 \multirow{3}{*}{6}  & TRUE & $x_4$ & $x_6$ & $x_5$ & -     & 5 & 7 & \\ \cline{2-9}
                     & TRUE & $x_4$ & -     & -     & -     & 7 & 7 & (c,b,[5,7),$r_2$,-)\\ \cline{2-9}
                     & TRUE & $x_4$ & -     & -     & $x_6$ & 7 & 7 & \\ \specialrule{1.2pt}{0pt}{0pt}
 
 \multirow{5}{*}{7}  & FALSE & $x_4$ & $x_7$ & -     & $x_6$ & 7 & 9 & - \\ \cline{2-9}
                     & TRUE  & $x_4$ & -     & -     & -     & 9 & 9 & - \\ \cline{2-9}
                     & TRUE  & $x_4$ & -     & $x_7$ & -     & 1 & 1 & - \\ \cline{2-9}
                     & TRUE  & $x_7$ & -     & -     & $x_7$ & 1 & 3 & - \\ 
                     & TRUE  & $x_7$ & -     & -     & -     & 3 & 3 & (d,b,[1,3),$r_3$,-) \\ \specialrule{1.2pt}{0pt}{0pt}
 \end{tabular}}
 \vspace*{0.5cm}
 \caption{The evolution of the  \emph{LIR$_{algo}$}-structure during the execution of the algorithm. The columns
 sP and bP refer to the sweepPoint and the breakPoint respectively.} 
 \label{tab:LIRexecution}
 \end{table}
 \end{center}

\subsection{Proof of Lemma~\ref{lem:secondObservation}}

\begin{lemma}
Assume two temporal probabilistic relations ${\bf r}$ and ${\bf s}$ with
schema $(F, T, \lambda)$ and the set of the base tuples $L_{b}(\lambda)$
in lineage expression $\lambda$. All the facts included in tuples of $LIR
({\bf r},{\bf s})$ are also included, during the same intervals, in
tuples of ${\bf r} \cup {\bf s}$ and vice versa.

\vspace*{0.2cm}
% {\centering \noindent $\exists k \in {\bf k} \ (k.F=f \ \wedge
% \ k.T = T_\kat{F} \ \wedge \ \lambda_\kat{F} = \lambda_{fun}(\lambda_1,\lambda_2))$}
\centering{$\pi_{F,T,L_{b}(\mathtt{\lambda_r}) \cup L_{b}(\mathtt{\lambda_s})  }(LIR({\bf r},{\bf s}))
\equiv \pi_{F,T,L_{b}(\lambda)}({\bf r}\cup^\kat{TP}{\bf s})$}
\end{lemma}

\vspace*{0.1cm}
\begin{proof}
For this equivalence to hold, all tuples in $\pi_{F,T,L_{b}(\lambda)}({\bf r}\cup^
\kat{TP}{\bf s})$ should belong to $\pi_{F,T,L_{b}(\mathtt{\lambda_r})\cup L_{b}(\mathtt{\lambda_s})}
(LIR({\bf r},{\bf s}))$ and vice versa. This requires both $\forall u \in \pi_{F,T,L_{b}(\mathtt{\lambda_r})
\cup L_{b}(\mathtt{\lambda_s})  }(LIR({\bf r},{\bf s}))\ (u \in \pi_{F,T}$\  $_{L_{b}(\lambda)}({\bf r}
\cup^\kat{TP}{\bf s}))$ and $\forall u \in \pi_{F,T,L_{b}(\lambda)}({\bf r}\cup^
\kat{TP}{\bf s})\ (u \in \pi_{F,T}$ $_{,L_{b}(\mathtt{\lambda_r}) \cup L_{b}(\mathtt{\lambda_s})}(LIR({\bf r},
{\bf s})))$ to hold. We will only focus on the first statement while the second one can be
proven in a similar fashion. We will assume that $\exists u \in \pi_{F,T,L_{b}(\mathtt{\lambda_r})
\cup L_{b}(\mathtt{\lambda_s})  }(LIR({\bf r},{\bf s}))\ (u \notin \pi_{F,T,L_{b}(\lambda)}
({\bf r}\cup^\kat{TP}{\bf s}))$ and show that it leads to contradiction.

%Relations $\pi_{F,T,L_{b}(\lambda)/\lambda_{set}}({\bf r}\cup^\kat{TP}
%{\bf s})$ and $\pi_{F,T,L_{b}(\lambda)/\lambda_{set}}({\bf r}\cap^
%\kat{TP}{\bf s})$ include all the tuples in ${\bf r}\cup^\kat{TP}{\bf s}$
%and ${\bf r}\cup^\kat{TP}{\bf s}$, after their lineage expressions have been
%replaced by the corresponding set of base tuples $L_b(\lambda)$. Consequently,
%each tuple in these relations

Assume tuple $u \in \pi_{F,T,L_{b}(\lambda)/\lambda_{set}}(LIR({\bf r},{\bf s}))$.
As all tuples in this relation, $u$ has been derived from a tuple $u' \in \ (LIR({\bf r},
{\bf s}))$ with $u'.F = u.F \wedge u'.T = u.T \wedge L_{b}(\mathtt{\lambda_r}) \cup L_{b}(\mathtt{\lambda_s}) 
= u.\lambda_{set}$. Given that $u$ and $u'$ include the same fact and interval, it holds
that $r_u = r_{u'} \wedge s_u = s_{u'}$. Moreover, since $u'$ belongs to the
result of {\bf LIR}, according to Definition~\ref{def:LIR}, it satisfies the
corresponding interval condition $i_c(u')$ and one of the pairs of fact and lineage
conditions in Table~\ref{tab:LIRCond}. Without loss of generality, we assume that
u satisfies the pair $r_{u'} \ne \mathtt{null} \wedge s_{u'} \ne \mathtt{null}$ and that
$u'.\mathtt{\lambda_r} = r_{u'}.\lambda \wedge u'.\mathtt{\lambda_s} = s_{u'}.\lambda$. Consequently,
given that $r_u = r_{u'} \wedge s_u = s_{u'}$, $u$ satisfies the above three conditions and
its lineage set can be rewritten as $u.\lambda_{set} = L_{b}(r_{u}.\lambda) \cup
L_{b}(s_{u}.\lambda)$.
%Also, by ignoring the logical operators, the set of base tuples included in
%$u.\lambda_{set}$ is equal to  
%$L_{b}(u'.\lambda) = L_{b}(r_{u'}.\lambda \cdot s_{u'}.\lambda) = L_b(r_{u}.\lambda))
%\cup L_b(s_{u}.\lambda)$. 

According to our initial assumption, $u \notin \pi_{F,T,L_{b}(\lambda)/
\lambda_{set}}({\bf r}\cup^\kat{TP}{\bf s})$. This means that $u$ cannot
have been derived from any tuple in ${\bf r}\cup^\kat{TP}{\bf s}$. So,
for all tuples $u''$ over the schema (F,T,$\lambda$,p) with $u'.F = u.F \wedge
u'.T = u.T \wedge L_{b}(u''.\lambda) = u.\lambda_{set}$, we conclude that $u''
\notin {\bf r}\cup^\kat{TP}{\bf s}$. Given that $u$ and $u'$ include the
same fact and interval, it holds that $r_u = r_{u''} \wedge s_u = s_{u''}$.  
Also, given the interval and fact condition satisfied by $u$, it holds that $u''$
satisfies the interval condition and $r_{u''} \ne \mathtt{null} \wedge s_{u''} \ne \mathtt{null}$.
However, $u''\notin {\bf r}\cup^\kat{TP}{\bf s}$. For this to hold, based on
Table~\ref{def:TPsetOps} and the interval and fact conditions that $u''$ satisfies,
$u''.\lambda \neq r_{u''}.\lambda \cdot s_{u''}.\lambda$. As a consequence
$L_{b}(u''.\lambda) \neq L_b(r_{u''}.\lambda) \cup L_b(s_{u''}.\lambda) \neq
L_b(r_{u}.\lambda) \cup L_b(s_{u}.\lambda)$. This contradicts our assumption
that $L_{b}(u''.\lambda) = u.\lambda_{set}$ prooving that $u \notin \pi_{F,T,L_{b}
(\lambda)/\lambda_{set}} ({\bf r}\cup^\kat{TP}{\bf s})$ is false, and thus
$\pi_{F,T,L_{b} (\lambda)}(LIR({\bf r},{\bf s})) \supseteq
\pi_{F,T,L_{b}(\lambda)} ({\bf r}\cup^\kat{TP}{\bf s})$.
\end{proof}

\subsection{Example LIR/set difference}

\begin{figure*}[t]
\begin{subfigure}[b]{0.3\linewidth}
\vspace*{0.2cm}
\centering 
\scalebox{0.8} {
\begin{tabular}{ c c c | c | c | c }
% \multicolumn{6}{l}{\bf \ \ \ \ \ \ \ R (productsWantedInHB)}\\
\multicolumn{6}{l}{\bf \ \ \ \ \ \ \ r (productsWanted)}\\
\cline{2-6} 
$k$   & $P$ &$B$  &  $T$      & $\lambda$ &  $p$  \\ \cline{2-6} %& $\lambda$
$r_1$ & m   & b   & {[2,10)} & $r_1$    & {0.3} \\%& $A_1$ 
$r_2$ & c   & b   & {[4,7)}  & $r_2$     & {0.2} \\%& $A_3$ 
$r_3$ & d   & b   & {[1,3)}  & $r_3$     & {0.4} \\%& $A_2$ 
\cline{2-6}
\end{tabular}}
%\hfill
\vspace*{0.3cm}

\scalebox{0.8} {
\begin{tabular}{ c c c | c | c | c }
\multicolumn{6}{l}{\bf \ \ \ \ \ \ \ s (productsInStock)}\\
\cline{2-6}   
$k$   & $P$ &$B$  &  $T$      & $\lambda$ &  $p$  \\ \cline{2-6} %& $\lambda$
$s_1$ & m   & b   & [1,4)   & $s_1$     & {0.6} \\%& $A_1$ 
$s_2$ & m   & b   & [6,8)   & $s_2$     & {0.3} \\%& $A_1$ 
$s_3$ & c   & b   & [4,5)   & $s_3$     & {0.7} \\%& $A_3$ 
$s_4$ & c   & b   & [7,9)   & $s_4$     & {0.1} \\%& $A_3$ 
\cline{2-6}
\end{tabular}}
\caption{Input Relations}
\label{fig:tpdb}
\end{subfigure}
\hfill
\begin{subfigure}[b]{0.34\linewidth}
\centering
\scalebox{0.8} {
\begin{tabular}{ c c | c | c | c }
\multicolumn{5}{l}{$LIR({\bf r},{\bf s})$}\\
\hline                                                       
$P$  & $B$  & $T$    & $\mathtt{\lambda_r}$ & $\mathtt{\lambda_s}$  \\ \hline %& $\lambda$
m    & b    & [1,2)  & -           & $s_1$ \\%& $A_1$ 
m    & b    & [2,4)  & $r_1$       & $s_1$ \\%& $A_1$ 
m    & b    & [4,6)  & $r_1$       &   -    \\%& $A_1$ 
m    & b    & [6,8)  & $r_1$       & $s_2$ \\%& $A_1$ 
m    & b    & [8,10) & $r_1$       &   -    \\%& $A_1$ 
c    & b    & [4,5)  & $r_2$       & $s_3$ \\%& $A_3$ 
c    & b    & [5,7)  & $r_2$       &   -    \\%& $A_3$ 
c    & b    & [7,9)  & -           & $s_3$    \\%& $A_3$ 
d    & b    & [1,3)  & $r_3$       &   -    \\%& $A_2$ 
\hline
\end{tabular}}
\caption{The Temporal Bi-lineage Relation of ${\bf LIR}({\bf r},{\bf s})$}
\label{tab:tpdbLIR}
\end{subfigure}
\hfill
\begin{subfigure}[b]{0.3\linewidth}
\vspace*{0.2cm}
\centering 
\scalebox{0.8} {
\begin{tabular}{ c c | c | c | c }
\multicolumn{5}{l}{${\bf u} = {\bf r} - ^\kat{TP} {\bf s}$}\\
\hline
$P$  & $B$  & $T$    & $\lambda$           & $p$ \\ \hline %& $\lambda$
m    & b    & [2,4)  & $r_1 \cdot !\ s_1$  & 0.12 \\ 
m    & b    & [4,6)  & $r_1$               & 0.3 \\ 
m    & b    & [6,8)  & $r_1 \cdot !\ s_2$  & 0.21 \\ 
m    & b    & [8,10) & $r_1$               & 0.3 \\ 
c    & b    & [4,5)  & $r_2 \cdot !\ s_3$  & 0.6 \\ 
c    & b    & [5,7)  & $r_2$               & 0.2 \\ 
d    & b    & [1,3)  & $r_3$               & 0.4 \\ 
\hline
\end{tabular}}
\caption{TP Set Difference}
\label{fig:tpdbDif}
\end{subfigure}

\vspace*{0.3cm}
\caption{The Supermarket Application Scenario}
\label{fig:tpdbResultConsecutive}
\end{figure*}

\subsection{Example Consecutive Operations}

\subsection{Example Sequenced VS Nonsequenced}

\begin{figure*}[t]
\begin{subfigure}[b]{0.3\linewidth}
\vspace*{0.2cm}
\centering 
\scalebox{0.8} {
\begin{tabular}{ c c c | c | c | c }
% \multicolumn{6}{l}{\bf \ \ \ \ \ \ \ R (productsWantedInHB)}\\
\multicolumn{6}{l}{\bf \ \ \ \ \ \ \ r (productsWanted)}\\
\cline{2-6} 
$k$   & $P$ &$B$  &  $T$      & $\lambda$ &  $p$  \\ \cline{2-6} %& $\lambda$
$r_1$ & m   & b   & {[2,10)} & $r_1$    & {0.3} \\%& $A_1$ 
$r_2$ & c   & b   & {[4,7)}  & $r_2$     & {0.2} \\%& $A_3$ 
$r_3$ & d   & b   & {[1,3)}  & $r_3$     & {0.4} \\%& $A_2$ 
\cline{2-6}
\end{tabular}}
%\hfill
\vspace*{0.3cm}

\scalebox{0.8} {
\begin{tabular}{ c c c | c | c | c }
\multicolumn{6}{l}{\bf \ \ \ \ \ \ \ s (productsInStock)}\\
\cline{2-6}   
$k$   & $P$ &$B$  &  $T$      & $\lambda$ &  $p$  \\ \cline{2-6} %& $\lambda$
$s_1$ & m   & b   & [1,4)   & $s_1$     & {0.6} \\%& $A_1$ 
$s_2$ & m   & b   & [6,8)   & $s_2$     & {0.3} \\%& $A_1$ 
$s_3$ & c   & b   & [4,5)   & $s_3$     & {0.7} \\%& $A_3$ 
$s_4$ & c   & b   & [7,9)   & $s_4$     & {0.1} \\%& $A_3$ 
\cline{2-6}
\end{tabular}}
\caption{Input Relations}
\label{fig:tpdbExfour}
\end{subfigure}
\hfill
\begin{subfigure}[b]{0.3\linewidth}
\vspace*{0.2cm}
\centering 
\scalebox{0.8} {
\begin{tabular}{ c c | c | c | c }
\multicolumn{5}{l}{${\bf u} = {\bf r} - ^\kat{TP} {\bf s}$}\\
\hline
$P$  & $B$  & $T$    & $\lambda$           & $p$ \\ \hline %& $\lambda$
m    & b    & [2,4)  & $r_1 \cdot !\ s_1$  & 0.12 \\ 
m    & b    & [4,6)  & $r_1$               & 0.3 \\ 
m    & b    & [6,8)  & $r_1 \cdot !\ s_2$  & 0.21 \\ 
m    & b    & [8,10) & $r_1$               & 0.3 \\ 
c    & b    & [4,5)  & $r_2 \cdot !\ s_3$  & 0.6 \\ 
c    & b    & [5,7)  & $r_2$               & 0.2 \\ 
d    & b    & [1,3)  & $r_3$               & 0.4 \\ 
\hline
\end{tabular}}
\caption{TP Set Difference}
\label{fig:difRSr}
\end{subfigure}
\hfill
\begin{subfigure}[b]{0.3\linewidth}
\vspace*{0.2cm}
\centering 
\scalebox{0.8} {
\begin{tabular}{ c c | c | c | c }
\multicolumn{5}{l}{${\bf u} = {\bf r} - ^\kat{TP} {\bf s}$}\\
\hline
$P$  & $B$  & $T$    & $\lambda$           & $p$ \\ \hline %& $\lambda$
m    & b    & [2,4)  & $r_1 \cdot !\ s_1$  & 0.12 \\ 
m    & b    & [4,6)  & $r_1$               & 0.3 \\ 
m    & b    & [6,8)  & $r_1 \cdot !\ s_2$  & 0.21 \\ 
m    & b    & [8,10) & $r_1$               & 0.3 \\ 
c    & b    & [4,5)  & $r_2 \cdot !\ s_3$  & 0.6 \\ 
c    & b    & [5,7)  & $r_2$               & 0.2 \\ 
d    & b    & [1,3)  & $r_3$               & 0.4 \\ 
\hline
\end{tabular}}
\caption{TP Set Difference}
\label{fig:difRSr}
\end{subfigure}

\vspace*{0.3cm}
\caption{Sequenced VS Nonsequenced}
\label{fig:tpdbResultr}
\end{figure*}

%
%Proof that the LIR and the Normalize lead to the same result
%
%Explain that the join of the normalizations leads in a temporal
%bi-lineage relation
%
%\begin{table}[ht]
%        \center
%\scalebox{0.9}{
%\begin{tabular}{|M{1.1cm}|M{1.5cm}|M{1.5cm}|M{4.2cm}| @{}m{0pt}@{}}
%  \hline
%  Op & f-Condition & $\lambda$-condition & Interval condition & \\
%  \hline
%  \multirow{2}{*}{$\mathcal{N}^\kat{$\lambda$}(r;s)$}
%  & \multirow{2}{*}{$r_\kat{F} \ne \mathtt{null}$}
%  & \multirow{2}{*}{\~r$.\lambda = r_\kat{F}.\lambda$}
%  & $\forall T'  \supset$ \ \~r$.T $ & \\[0.12cm]
%  
%  & &
%  & $(O({\bf r},$\~r.$F,$\~r$.T) \ne  O({\bf r},$\~r.$F,T')$ & \\[0.12cm] \cline{1-3}
%  %%%%%%%%%%%%%%%%%%%%%%%%%%%%%%%%%%%%%%%%%%%%%%%%%%%%%%%%%%%%%%%%%%%%%%%%%%%%%%%%%%%%%%%%%%%%%%%%%%%%%%%%%%%%%%%%
%  \multirow{3}{*}{$\mathcal{N}^\kat{$\lambda$}(s;r)$}
%  & \multirow{3}{*}{ $s_\kat{F} \ne \mathtt{null}$}
%  & \multirow{3}{*}{\~s$.\lambda = s_\kat{F}.\lambda$}
%  & $\vee \ O({\bf s},$\~r.$F,$\~r$.T) \ne O({\bf s},$\~r.$F,T')$ & \\[0.12cm] 
%  
%  & &
%  &  $\vee\  \{r_\kat{F}\} \ne  I({\bf r},$\~r.$F,T')$  & \\[0.12cm] 
%  
%  & &
%  &   $\vee \ \{s_\kat{F}\} \ne I({\bf s},$\~r.$F,T')\ )$ & \\[0.12cm] \hline 
%\end{tabular}}
%\vspace{0.2cm}
%\caption{Equivalence}
%\label{tab:equivNLIR}
%\end{table}

\subsection{Previous Intro Example}

\begin{figure}[htb]
\scalebox{0.52} {
\begin{tikzpicture}   
% x - axis
\draw (0,0) [->, line width = 1pt]-- coordinate (x axis mid) (15.5,0);
\node[font=\relsize{2.5}] at (15.5,0.3) {${\bf t}$}; %[2,10)
% \draw (0.5,1.3) [line width = 1pt,dashed]-- coordinate (x axis mid) (16.5,1.3);

\pgfmathsetmacro{\shift}{0.5}
\foreach \j in {1,...,11}{
     \pgfmathsetmacro{\divRes}{int(\j/2)}
     \pgfmathsetmacro{\modRes}{1-(\j-\divRes*2)}
     \pgfmathsetmacro{\xPos}{\j-1+(\divRes-\modRes*\shift)}
     \draw (\xPos , 1pt)  --  (\xPos ,-3pt) node[anchor=north,font=\relsize{2}] {};
}

\pgfmathsetmacro{\shift}{0.5}
\foreach \j in {1,...,10}{
     \pgfmathsetmacro{\divRes}{int(\j/2)}
     \pgfmathsetmacro{\modRes}{1-(\j-\divRes*2)}
     \pgfmathsetmacro{\xPos}{\j-1+(\divRes-\modRes*\shift)}
     \draw (\xPos+0.75 , -3pt) node[anchor=north,font=\relsize{2}] {\bf \j};
}

%tuples referring to (a,b) in r,s
\draw [line width=1.2,font=\relsize{2.5},color=c1] (1.5, 1.5) -- (13.5, 1.5) node[pos=.5,above=-1pt]{$(m,b,r_1)$};%[2,10)   
%\draw (2.5, 1.6) node[anchor=north,fill=black] {};
\draw [line width=1.2,font=\relsize{2.5},color=c3] (0, 0.5) -- (4.5, 0.5) node[pos=.5,above=-1pt]{$(m,b,s_1)$}; %[1,5)
%\draw (1, 0.6) node[anchor=north,fill=black] {};
\draw [line width=1.2,font=\relsize{2.5},color=c3] (7.5, 0.5) -- (10.5,0.5) node[pos=.5,above=-1pt]{$(m,b,s_2)$}; %[6,8]
%\draw (8.5, 0.6) node[anchor=north,fill=black] {};

%adjusted tuples referring to (a,b)
\draw [line width=1.2,font=\relsize{2.5}] (0   ,-2.2)  -- (1.5, -2.2)  node[pos=.5,above=-1pt]{$(m,b,-  ,s_1)$};
\draw [line width=1.2,font=\relsize{2.5}] (1.5 ,-1.4)  -- (4.5, -1.4)  node[pos=.5,above=-1pt]{$(m,b,r_1,s_1)$};
\draw [line width=1.2,font=\relsize{2.5}] (4.5 ,-2.2)  -- (7.5, -2.2)  node[pos=.5,above=-1pt]{$(m,b,r_1,-  )$};
\draw [line width=1.2,font=\relsize{2.5}] (7.5 ,-1.4)  -- (10.5,-1.4) node[pos=.5,above=-1pt]{$(m,b,r_1,s_2)$};
\draw [line width=1.2,font=\relsize{2.5}] (10.5,-2.2)  -- (13.5,-2.2) node[pos=.5,above=-1pt]{$(m,b,r_1,-  )$};

\end{tikzpicture}}
\vspace*{0.4cm}
\caption{$LIR(\{r_1\},\{s_1,s_2\})$}
\label{fig:LIRexample}
\end{figure}

%the LIR allows gathers all the tuples that will contribute in the result
and it also groups the time-points in a way that the changes in the valid tuples 
are recorded. Thus is guarantees that the intervals in the output will respect
snapshot reducibility and change preservation. 

The final result is produced simply by applying filtering and lineage bla bla in the temporal
bilineage relation produced by the LIR.

In Fig.~\ref{fig:LIRexample}, we illustrate the temporal bilineage relation produced
by the Lineage Time Adaptor

 how $LIR$ combines the information
of the tuples in relations ${\bf r}$ and ${\bf s}$ (Fig.~\ref{fig:tpdbEx})
that include fact $(m,b)$. 

%At time-point $t=3$, the fact \emph{(m,b)} is included
in tuple $r_1$ of ${\bf r}$ and in tuple $s_1$ of ${\bf s}$. The same
holds for time-point $t=2$ but doesn't hold for time-point $t=4$ and thus, the
tuple \emph{(m,b,[2,4), $r_1$, $s_1$)} is added in the {\bf LIR} result with
$r_1$ and $s_1$ being the lineage expressions of the corresponding tuples.  

At
time-point $t=1$, the fact \emph{(m,b)} is only included in a tuple of ${\bf s}$
and this leads to the tuple \emph{(m,b, [1,2), $-$, $s_1$)}.  Comparing the
result of {\bf LIR} with the result of TP set difference, tuple \emph{(m,b, [2,4), 
$r_1$, $s_1$)} can be transformed to tuple \emph{(m,b, [2,4), $r_1 \cdot ! s_1$)}
after the lineage expressions $\mathtt{\lambda_s} = r_1.\lambda =  r_1$ and $\mathtt{\lambda_s} =
s_1.\lambda = s_1$ are combined $r_1 \cdot ! s_1$. On the other hand, the is no
tuple in the result of TP set difference carrying equivalent information with tuple
\emph{(m,b, [1,2), $-,s_1$)} of {\bf LIR}.

%According to tuple
\emph{(m, [2,4), $r_1 \cdot ! s_1$, 0.12)} in ${\bf r}-^\kat{TP} {\bf s}$,
fact \emph{m} is wanted and is not in stock at each time-point in the interval $[2,4)$
with probability $0.12$. The lineage expression $r_1 \cdot ! s_1$ is a conjuction of
($\cdot$)  between the lineage of tuple $r_1$ and the negated ($!$) lineage of $s_1$. 
As it is reflected in the lineage expression, in ${\bf r}-^\kat{TP} {\bf s}$, fact
\emph{(m)} is $\mathit{true}$ during $[2,4)$ if tuple $r_1$ is $\mathit{true}$ and
tuple $s_1$ is $\mathit{false}$. Its truth over the time-points in $[2,4)$ depends 
only on tuples $r_1$ and $s_1$ given that they are the only tuples whose interval
overlaps with $[2,4)$ and that they include fact \emph{(m)}.  Similarly,
the existence of the output tuple \emph{(m,b, [4,6), $r_1$, 0.3)} in
${\bf r}-^\kat{TP} {\bf s}$ is only attributed to $r_1$ since no
other tuple includes fact \emph{(m,b)} during interval $[4,6)$. Although tuples 
\emph{(m, [2,4), $r_1 \cdot ! s_1$, 0.12)} and \emph{(m,b, [4,6), $r_1$, 0.3)}
include the same fact over consecutive time-points, their intervals cannot be coalesced
since the corresponding lineage expressions and thus the probability with which
\emph{m} is $\it{true}$ differs.

  We use green for
  the tuples in ${\bf r}$, red for the tuples in ${\bf s}$
  that include $(m,b)$.  We use black for the tuples of the temporal
  bilineage relation with schema ($F$, $T$, $\mathtt{\lambda_r}$, $\mathtt{\lambda_s}$)
  resulting from ${\bf LIR}({\bf r},{\bf s})$ with
  $F=(m,b)$. 
  
  \begin{tikzpicture}
\node at (0,2.3) {
\scalebox{0.8} {
\begin{tabular}{ c c | c | c | c }
% \multicolumn{6}{l}{\bf \ \ \ \ \ \ \ R (productsWantedInHB)}\\
\multicolumn{5}{l}{\bf \ \ \ \ \ \ \ r (productsWanted)}\\
\cline{2-5} 
$k$   & $P$ &  $T$      & $\lambda$ &  $p$  \\ \cline{2-5} %& $\lambda$
\color{red}{$r_1$} & \color{red}{m} & \color{red}{[2,10)} & \color{red}{$r_1$} & \color{red}{0.3} \\ 
$r_2$ & c   & {[4,7)}  & $r_2$     & {0.2} \\%& $A_3$ 
\color{green}{$r_3$} &\color{green}{d} &\color{green}{[1,3)} & \color{green}{$r_3$} & \color{green}{0.4} \\
\cline{2-5}
\end{tabular}}};

\node at (0,0) {
\scalebox{0.8} {
\begin{tabular}{ c c | c | c | c }
\multicolumn{5}{l}{\bf \ \ \ \ \ \ \ s (productsInStock)}\\
\cline{2-5}   
$k$   & $P$ &  $T$    & $\lambda$ &  $p$  \\ \cline{2-5} 
\color{red}{$s_1$} & \color{red}{m} & \color{red}{[1,4)} & \color{red}{$s_1$} & \color{red}{0.6} \\
\color{red}{$s_2$} & \color{red}{m} & \color{red}{[6,8)} & \color{red}{$s_2$} & \color{red}{0.3} \\ 
$s_3$ & c   & [4,5)   & $s_3$     & {0.7} \\%& $A_3$ 
$s_4$ & c   & [7,9)   & $s_4$     & {0.1} \\%& $A_3$ 
\cline{2-5}
\end{tabular}}};

\node at (4.5,1.1) {
\scalebox{0.8} {
\begin{tabular}{ c | c | c | c }
\multicolumn{4}{l}{$LIR({\bf r},{\bf s})$}\\
\hline                                                       
$P$  & $T$    & $\mathtt{\lambda_r}$ & $\mathtt{\lambda_s}$  \\ \hline 
m    & [1,2)  & -           & $s_1$ \\%& $A_1$ 
m    & [2,4)  & $r_1$       & $s_1$ \\%& $A_1$ 
m    & [4,6)  & $r_1$       &   -    \\%& $A_1$ 
m    & [6,8)  & $r_1$       & $s_2$ \\%& $A_1$ 
m    & [8,10) & $r_1$       &   -    \\%& $A_1$ 
c    & [4,5)  & $r_2$       & $s_3$ \\%& $A_3$ 
c    & [5,7)  & $r_2$       &   -    \\%& $A_3$ 
c    & [7,9)  & -           & $s_3$    \\%& $A_3$ 
d    & [1,3)  & $r_3$       &   -    \\%& $A_2$ 
\hline
\end{tabular}}};
\end{tikzpicture}

\begin{figure}[htbp]
%\begin{subfigure}[b]{0.48\linewidth}
\vspace*{0.2cm}
\centering 
\scalebox{0.8} {
\begin{tabular}{ c c c | c | c | c }
% \multicolumn{6}{l}{\bf \ \ \ \ \ \ \ R (productsWantedInHB)}\\
\multicolumn{6}{l}{\bf \ \ \ \ \ \ \ r (productsWanted)}\\
\cline{2-6} 
$k$   & $P$ &$B$  &  $T$      & $\lambda$ &  $p$  \\ \cline{2-6} %& $\lambda$
$r_1$ & m   & b   & {[2,10)} & $r_1$    & {0.3} \\%& $A_1$ 
$r_2$ & c   & b   & {[4,7)}  & $r_2$     & {0.2} \\%& $A_3$ 
$r_3$ & d   & b   & {[1,3)}  & $r_3$     & {0.4} \\%& $A_2$ 
\cline{2-6}
\end{tabular}}
\hfill
%\vspace*{0.3cm}
\scalebox{0.8} {
\begin{tabular}{ c c c | c | c | c }
\multicolumn{6}{l}{\bf \ \ \ \ \ \ \ s (productsInStock)}\\
\cline{2-6}   
$k$   & $P$ &$B$  &  $T$      & $\lambda$ &  $p$  \\ \cline{2-6} %& $\lambda$
$s_1$ & m   & b   & [1,4)   & $s_1$     & {0.6} \\%& $A_1$ 
$s_2$ & m   & b   & [6,8)   & $s_2$     & {0.3} \\%& $A_1$ 
$s_3$ & c   & b   & [4,5)   & $s_3$     & {0.7} \\%& $A_3$ 
$s_4$ & c   & b   & [7,9)   & $s_4$     & {0.1} \\%& $A_3$ 
\cline{2-6}
\end{tabular}}
\vspace*{0.2cm}
\caption{Input Relations}
\label{fig:tpdbEx}
\end{figure}

%\end{subfigure}
\hfill
\begin{subfigure}[b]{0.55\linewidth}
\vspace*{0.2cm}
\centering 
\scalebox{0.8} {
\begin{tabular}{ c c | c | c | c }
\multicolumn{5}{l}{${\bf r} - ^\kat{TP} {\bf s}$}\\
\hline
$P$  & $B$  & $T$    & $\lambda$           & $p$ \\ \hline %& $\lambda$
m    & b    & [2,4)  & $r_1 \cdot !\ s_1$  & 0.12 \\ 
m    & b    & [4,6)  & $r_1$               & 0.3 \\ 
m    & b    & [6,8)  & $r_1 \cdot !\ s_2$  & 0.21 \\ 
m    & b    & [8,10) & $r_1$               & 0.3 \\ 
c    & b    & [4,5)  & $r_2 \cdot !\ s_3$  & 0.6 \\ 
c    & b    & [5,7)  & $r_2$               & 0.2 \\ 
d    & b    & [1,3)  & $r_3$               & 0.4 \\ 
\hline
\end{tabular}}
\caption{TP Set Difference}
\label{fig:difRS}
\end{subfigure}
\hfill
\vspace*{0.2cm}
\caption{The Supermarket Application Scenario}
\label{fig:tpdbResult}

\begin{figure}[!h]
\tikzset{%
  algebra/.style    = {draw, thick, rectangle, minimum height = 2em,
    minimum width = 2em},
}
\tikzset{%
  lineage/.style    = {draw, thick, rectangle, minimum height = 2em,
    minimum width = 2.3cm},
}
\tikzset{%
  filter/.style    = {draw, thick, rectangle, minimum height = 2em,
    minimum width = 2.75cm},
}
\tikzset{%
  block/.style    = {draw, thick, rectangle, minimum height = 2em,
    minimum width = 2em},
}
\centering
\scalebox{0.8}{
\begin{tikzpicture}[auto, thick, node distance=2cm, >=triangle 45, block1/.style    = {draw, thick, rectangle, minimum height = 3cm,
    minimum width = 2em}]
\draw
	% Drawing the blocks of first filter :
	node at (0,0)[right=-3mm] (relR) {{\bf R}}
	node [below = 0.6cm of relR] (relS) {{\bf S}}

	node [right =0.7cm of relR] (f1) {}
	node [right =0.7cm of relS]  (f2) {}

	node [below right = 0.21cm and 0.45cm of relR] (LIRNode) {}
	node [right = 0.1cm of LIRNode, block1] (LIR) {\color{c1}{LIR}}

	node [above right =0.35cm and 0.65cm of f1] (setD) {}
	node [below right =0.35cm and 0.65cm of f1] (setI) {}
	node [below right =0.35cm and 0.65cm of f2] (setU) {}

	node [right = 0.7cm of setI, filter] (filtI) {\color{c1}{$\lambda_R \ne \mathtt{null} \wedge \lambda_S \ne \mathtt{null}$)}}
	node [right = 0.7cm of setD, filter] (filtD) {\color{c2}{$\lambda_R \ne \mathtt{null}$}}
	node [right = 0.7cm of setU, filter,white] (filtU) {}

	node [right = 0.85cm of filtI, lineage] (setIL) {\color{c1}{and($\lambda_R$, $\lambda_S$)}}
	node [right = 0.85cm of filtD, lineage] (setDL) {\color{c2}{andNot($\lambda_R$, $\lambda_S$)}}
	node [right = 0.85cm of filtU, lineage] (setUL) {\color{c3}{or($\lambda_R$, $\lambda_S$)}}

	node [right =0.7cm of setIL] (resI) {\color{c1}{$ \bf{R} \cap^\kat{TP} \bf{S}$}}
	node [right =0.7cm of setDL] (resD) {\color{c2}{$ \bf{R} -^\kat{TP} \bf{S}$}}
	node [right =0.7cm of setUL] (resU) {\color{c3}{$ \bf{R} \cup^\kat{TP} \bf{S}$}};

\draw[->] (relR) -- (f1.center);
\draw[->] (relS) -- (f2.center);

\draw[->] (setI.west)  -- (filtI.west);
\draw[->] (filtI.east)  -- (setIL);

\draw[->] (setD.west) -- (filtD.west);
\draw[->] (filtD.east) -- (setDL);

\draw[->] (setU.west) -- (setUL);

\draw[->] (setIL.east) -- (resI);
\draw[->] (setDL.east) -- (resD);
\draw[->] (setUL.east) -- (resU);

\end{tikzpicture}}

\vspace{0.2cm}

\caption{LIR for TP Set Operations}
\label{fig:LIRTP}
\end{figure}

%%%%%%%%%%%%%%%%%%%%%%%%%%%%%%%%%%%%%%%%%%%%%%%%%%%%%%%%%%%%%%
 \begin{figure}[h]
 \begin{center}
 \scalebox{0.5} {
 \begin{tikzpicture}   
    % x - axis
    \draw (0.5,0) [->, line width = 1pt]-- coordinate (x axis mid) (16.5,0);
    %\draw (0.5,1.7) [line width = 1pt,dashed]-- coordinate (x axis mid) (16.5,1.7);
    
    \pgfmathsetmacro{\shift}{0.5}
    \foreach \j in {1,...,11}{
         \pgfmathsetmacro{\divRes}{int(\j/2)}
         \pgfmathsetmacro{\modRes}{1-(\j-\divRes*2)}
         \pgfmathsetmacro{\xPos}{\j+(\divRes-\modRes*\shift)}
         \draw (\xPos , 1pt)  --  (\xPos ,-3pt) node[anchor=north] {\bf \j};
    }

    %  TESTING VERTICALLY
    %  \draw (0,3) [->, line width = 1pt]-- coordinate (x axis mid) (16,3);  
    %   \foreach \j in {1,...,15}{
    %        \draw (\j, 3)  --  (\j ,3) node[anchor=north] {\bf \j};
    %   }
    %   \foreach \j in {1,...,15}{
    %           \draw[color=gray,dashed] (\j , 3)  --  (\j ,-3) ;
    %      }
       
    %tuples (\divRes-\modRes*\shift)
    %\draw [color=white]  (3, 2.1) -- (8, 2.1) node[pos=.5,above=-1pt]{$Nicely drawn$};
    %\node at (0.5,2.3) {${\bf r}$}; %[2,10)
    %\node at (0.5,0.7) {${\bf s}$}; %[2,10)
    \draw [line width=1.5,color=c1] (2.5, 2.7) -- (14.5, 2.7) node[pos=.5,above=-1pt]{$r_1$}; %[2,10)   
    \draw [line width=1.5,color=c3] (5.5, 2.1) -- (9.95, 2.1) node[pos=.5,above=-1pt]{$r_2$}; %[4,7)
    \draw [line width=1.5,color=c4] (1, 2.1) -- (4, 2.1) node[pos=.5,above=-1pt]{$r_3$}; %[1,3)
    
    \draw [line width=1.5,color=c1] (1, 1) -- (5.5,1) node[pos=.5,above=-1pt]{$s_1$}; %[1,4)
    \draw [line width=1.5,color=c1] (8.5, 1) -- (11.5,1) node[pos=.5,above=-1pt]{$s_2$}; %[6,8]
    \draw [line width=1.5,color=c3] (5.5, 0.4) -- (7,0.4) node[pos=.5,above=-1pt]{$s_3$}; %[4,5]
    \draw [line width=1.5,color=c3] (10.1, 0.4) -- (13,0.4) node[pos=.5,above=-1pt]{$s_4$}; %[7,10]
    
    %adjusted intervals - r3
    \draw [line width=1.5,color=c4] (1,-1.2) -- (4,-1.2) node[pos=.5,above=-1pt]{$r_3$};
    
    %adjusted intervals - r1
    %\node at (0.5,-1.7) {${\bf r}-^\kat{TP}{\bf s}$}; %[2,10)
    \draw [line width=1.5,color=c1] (2.5, -1.7) -- (5.5,-1.7) node[pos=.5,above=-1pt]{$r_1 \wedge \lnot s_1$};
    \draw [line width=1.5,color=c1] (5.5,-1.2) -- (8.5,-1.2) node[pos=.5,above=-1pt]{$r_1$};
    \draw [line width=1.5,color=c1] (8.5,-2.2) -- (11.5,-2.2) node[pos=.5,above=-1pt]{$r_1 \wedge \lnot s_2$};
    \draw [line width=1.5,color=c1] (11.5, -1.2) -- (14.5,-1.2) node[pos=.5,above=-1pt]{$r_1$};

    %adjusted intervals - r2
    \draw [line width=1.5,color=c3] (5.5,-2.2) -- (7,-2.2) node[pos=.5,above=-1pt]{$r_2 \wedge \lnot s_3$};
    \draw [line width=1.5,color=c3] (7,-1.7) -- (10,-1.7) node[pos=.5,above=-1pt]{$r_2$};

 \end{tikzpicture}}
 \end{center}
 
 \caption{Temporal Probabilistic Set Difference ${\bf r}-^\kat{TP}{\bf s}$}
 \label{fig:tpdbSetDif}

\end{figure}

\begin{figure}[h]
\centering
\begin{tikzpicture}
\node at (0,1) {
\scalebox{0.85} {
\begin{tabular}{ M{0.8cm} | M{0.7cm} | M{0.2cm} @{}m{0pt}@{}}
\multicolumn{3}{l}{\bf r (productsWanted)}\\
\cline{1-3} 
$P$ &  $T$      & $\lambda$ & \\  \cline{1-3} %& $\lambda$
m    & {[2,10)} & {$r_1$} & \\ [0.1cm]
c     & {[4,7)}   & {$r_2$} & \\ [0.1cm]%& $A_3$ 
d     & {[1,3)}   & {$r_3$} & \\ [0.1cm]
\cline{1-3}
\multicolumn{3}{l}{}\\ [0.1cm]
%\end{tabular}}};
%
%
%
%\node at (0,0) {
%\scalebox{0.85} {
%\begin{tabular}{ M{0.8cm} | M{0.7cm} | M{0.2cm} @{}m{0pt}@{}}
\multicolumn{3}{l}{\bf s (productsInStock)}\\
\cline{1-3}   
$P$ &  $T$     & $\lambda$ & \\  \cline{1-3}  %& $\lambda$
m    & {[1,4)} & $s_1$  & \\ [0.1cm]
m    & {[6,8)} & $s_2$  &\\  [0.1cm]
c     & [4,5)    & $s_3$  & \\ [0.1cm]
c     & [7,9)    & $s_4$  & \\ [0.1cm] 
\cline{1-3}
\end{tabular}}};

%%groups in r
%\draw[line width=1,color=c3] (-1.23,2.46) -- (1.34,2.46) -- (1.34,2.73) -- (-1.23,2.73) -- (-1.23,2.46);
%\draw[line width=1,color=c2] (-1.23,2.06) -- (1.34,2.06) -- (1.34,2.37) -- (-1.23,2.37) -- (-1.23,2.06);
%\draw[line width=1,color=c1] (-1.23,1.66) -- (1.34,1.66) -- (1.34,1.95)      -- (-1.23,1.95)      -- (-1.23,1.66);
%
%%groups in s
%\draw[line width=1,color=c3] (-1.23,-0.03) -- (1.34,-0.03) -- (1.34,0.63)   -- (-1.23,0.63)  -- (-1.23,-0.03);
%\draw[line width=1,color=c2] (-1.23,-0.83) -- (1.34,-0.83) -- (1.34,-0.15)  -- (-1.23,-0.15) -- (-1.23,-0.83);

\path[draw=black,solid,line width=2mm,fill=black,
preaction={-triangle 90,thin,draw,shorten >=-1mm}
] (1.6, 1.2) -- (3.1, 1.2);

\node at (2.3, 1.45) {\tiny Lineage Time};
\node at (2.3, 0.9) {\tiny Adaptor};

\node at (4.5,1.3) {
\scalebox{0.8} {
\begin{tabular}{ M{0.3cm} | M{0.7cm} | M{0.3cm} | M{0.5cm} @{}m{0pt}@{}}
\multicolumn{4}{l}{$LIR(\mathbf{r},\mathbf{s})$}\\
\hline                                                       
$P$  & $T$     & $\mathtt{\lambda_r}$ & $\mathtt{\lambda_s}$  \\ \hline 
m    & [1,2)   & -        & $s_1$  &\\ [0.1cm]
m    & [2,4)   & $r_1$    & $s_1$  &\\ [0.1cm] 
m    & [4,6)   & $r_1$    &   -    &\\ [0.1cm]
m    & [6,8)   & $r_1$    & $s_2$  &\\ [0.1cm]
m    & [8,10)  & $r_1$    &   -    &\\ [0.1cm]
c    & [4,5)   & $r_2$    & $s_3$  &\\ [0.1cm]
c    & [5,7)   & $r_2$    &   -    &\\ [0.1cm]
c    & [7,9)   & -        & $s_3$  &\\ [0.1cm]
d    & [1,3)   & $r_3$    &   -    &\\ [0.1cm]
\hline
\end{tabular}}};

%groups in LIR
\draw[line width=1,color=c3] (3.3,0.85) -- (5.8,0.85) -- (5.8,2.63) -- (3.3,2.63) -- (3.3,0.85);
\draw[line width=1,color=c2] (3.3,-0.25) -- (5.8,-0.25) -- (5.8,0.78) -- (3.3,0.78) -- (3.3,-0.25);
\draw[line width=1,color=c1] (3.3,-0.65) -- (5.8,-0.65) -- (5.8,-0.32) -- (3.3,-0.32) -- (3.3,-0.65);

%% arrows from groups of r to LIR
%\draw[line width=1,color=c3,->] (1.6,2.6) -- (3.3,1.8);
%\draw[line width=1,color=c2,->] (1.6,2.27)-- (3.3,0.33);
%\draw[line width=1,color=c1,->] (1.6,1.9) -- (3.3,-0.5);
%
%% arrows from groups of s to LIR
%\draw[line width=1,color=c3,->] (1.6,0.3) -- (3.3,1.7);
%\draw[line width=1,color=c2,->] (1.6,-0.45) -- (3.3,0.2);
%\draw[line width=1,color=c1,->] (1.6,-1) -- (3.3,-0.88);

%\path[draw=black,solid,line width=2mm,fill=black,
%preaction={thin,draw,shorten >=-1mm}
%] (5.9, 1.2) -- (6.4, 1.2);
%
%\path[draw=black,solid,line width=2mm,fill=black,
%preaction={thin,draw,shorten >=-1mm}
%] (6.4, 1.1) -- (6.4, 2.4);
%
%\path[draw=black,solid,line width=2mm,fill=black,
%preaction={-triangle 90,thin,draw,shorten >=-1mm}
%] (6.3, 2.4)  -- (7.4, 2.4);

\path[draw=black,solid,line width=2mm,fill=black,
preaction={-triangle 90,thin,draw,shorten >=-1mm}
] (4.5, -1.2) -- (4.5, -2.15);

\node at (3.25, -1.6) {\tiny Lineage-Based Filtering};
\node at (3.25, -1.85){\tiny$(\mathtt{\lambda_r} \neq \mathtt{null}
\wedge \mathtt{\lambda_s} \neq \mathtt{null})$};

\node at (4.5, -3.3) {
\scalebox{0.8} {
\begin{tabular}{ M{0.3cm} | M{0.7cm} | M{0.3cm} | M{0.5cm} @{}m{0pt}@{}}
\hline                                                       
$P$  & $T$     & $\mathtt{\lambda_r}$ & $\mathtt{\lambda_s}$  \\ \hline 
m    & [2,4)    & $r_1$    & $s_1$  &\\ [0.1cm] 
m    & [6,8)    & $r_1$    & $s_2$  &\\ [0.1cm]
c    & [4,5)     & $r_2$    & $s_3$  &\\ [0.1cm]
\hline
\end{tabular}}};

\path[draw=black,solid,line width=2mm,fill=black,
preaction={-triangle 90,thin,draw,shorten >=-1mm}
] (3, -3.5) -- (1.7, -3.5);

\node at (2.4, -3) {\tiny Lineage};
\node at (2.4, -3.2) {\tiny Concatenation};

\node at (0.1, -3.15) {
\scalebox{0.8} {
\begin{tabular}{ M{0.3cm} | M{0.7cm} | M{0.75cm} @{}m{0pt}@{}}
\multicolumn{3}{l}{${\bf u} = {\bf r} \cap^\kat{T} {\bf s}$}\\
\hline
$P$  & $T$    & $\lambda$         \\ \hline %& $\lambda$
m    & [2,4)  & $r_1 \cdot \ s_1$ \\ [0.1cm] 
m    & [6,8)  & $r_1 \cdot \ s_2$ \\ [0.1cm]
c    & [4,5)  & $r_2 \cdot \ s_3$ \\ [0.1cm] 
\hline
\end{tabular}}};

\end{tikzpicture}
\vspace*{0.3cm}
\caption{Computation of a TP set operation using the LIR:
(a) Lineage-Enhanced Temporal Relations,
(b) The Temporal Bi-lineage Relation produced by $LIR({\bf r}, {\bf s})$,
(c) Lineage-Based Filtering
(d) Set Intersection}
\label{fig:LIRfullexample}
\end{figure}

\subsection{Anton}

\begin{figure}[h]
\centering
\begin{subfigure}[b]{0.6\linewidth}
\centering
\scalebox{0.8} {
\begin{tabular}{ M{0.3cm} | M{0.7cm} | M{0.2cm} @{}m{0pt}@{}}
\multicolumn{3}{l}{\bf r}\\
\cline{1-3} 
$P$ &  $T$      & $\lambda$ & \\  \cline{1-3} %& $\lambda$
m    & {[2,10)} & {$r_1$} & \\ [0.1cm]
c     & {[4,7)}   & {$r_2$} & \\ [0.1cm]%& $A_3$ 
d     & {[1,3)}   & {$r_3$} & \\ [0.1cm]
\cline{1-3}
\end{tabular}}
\qquad
\scalebox{0.8} {
\begin{tabular}{ M{0.3cm} | M{0.7cm} | M{0.2cm} @{}m{0pt}@{}}
\multicolumn{3}{l}{\bf s }\\
\cline{1-3}   
$P$ &  $T$     & $\lambda$ & \\  \cline{1-3}  %& $\lambda$
m    & {[1,4)} & $s_1$  & \\ [0.1cm]
m    & {[6,8)} & $s_2$  &\\  [0.1cm]
c     & [4,5)    & $s_3$  & \\ [0.1cm]
c     & [7,9)    & $s_4$  & \\ [0.1cm] 
\cline{1-3}
\end{tabular}}
\caption{}
\end{subfigure}
\qquad
\begin{subfigure}[b]{0.3\linewidth}
\centering
\scalebox{0.8} {
\begin{tabular}{ M{0.3cm} | M{0.7cm} | M{0.75cm} @{}m{0pt}@{}}
\multicolumn{3}{l}{${\bf r} \cap^\kat{T} {\bf s}$}\\
\hline
$P$  & $T$    & $\lambda$         \\ \hline %& $\lambda$
m    & [2,4)  & $r_1 \cdot \ s_1$ \\ [0.1cm] 
m    & [6,8)  & $r_1 \cdot \ s_2$ \\ [0.1cm]
c     & [4,5)  & $r_2 \cdot \ s_3$ \\ [0.1cm] 
\hline
\end{tabular}}
\caption{}
\end{subfigure}
\vspace{0.2cm}

\begin{subfigure}[b]{0.58\linewidth}
\centering
\scalebox{0.8} {
\begin{tabular}{ M{0.3cm} | M{0.7cm} | M{0.3cm}  @{}m{0pt}@{}}
\multicolumn{4}{l}{$N(\mathbf{r},\mathbf{s})$}\\
\hline                                                       
$P$  & $T$     & $\lambda$ \\ \hline 
m    & [2,4)   & $r_1$ &\\ [0.1cm] 
m    & [4,6)   & $r_1$ &\\ [0.1cm]
m    & [6,8)   & $r_1$ &\\ [0.1cm]
m    & [8,10) & $r_1$ &\\ [0.1cm]
c     & [4,5)   & $r_2$ &\\ [0.1cm]
c     & [5,7)   & $r_2$ &\\ [0.1cm]
d     & [1,3)   & $r_3$ &\\ [0.1cm]
\hline
\end{tabular}}
\qquad
\scalebox{0.8} {
\begin{tabular}{ M{0.3cm} | M{0.7cm} | M{0.3cm} @{}m{0pt}@{}}
\multicolumn{4}{l}{$N(\mathbf{s},\mathbf{r})$}\\
\hline                                                       
$P$  & $T$   & $\mathtt{\lambda_s}$   \\ \hline 
m    & [1,2)  & $s_1$  &\\ [0.1cm]
m    & [2,4)  & $s_1$  &\\ [0.1cm] 
m    & [6,8)  & $s_2$  &\\ [0.1cm]
c     & [4,5)   & $s_3$  &\\ [0.1cm]
c     & [7,9)   & $s_3$  &\\ [0.1cm]
\hline
\end{tabular}}
\caption{}
\end{subfigure}
\qquad
\begin{subfigure}[b]{0.32\linewidth}
\centering
\scalebox{0.8} {
\begin{tabular}{ M{0.3cm} | M{0.7cm} | M{0.65cm} | M{0.65cm} @{}m{0pt}@{}}
\multicolumn{4}{l}{${\bf u} = \mathcal{N}(r;s) \ \Join\theta \ \mathcal{N}(s;r)$}\\
\hline
$P$  & $T$   & $r.\lambda$ & $s.\lambda$  \\ \hline %& $\lambda$
m    & [2,4)  & $r_1 $ & $s_1$ \\ [0.1cm] 
m    & [6,8)  & $r_1 $ & $s_2$ \\ [0.1cm]
c     & [4,5)  & $r_2$  & $s_3$ \\ [0.1cm] 
\hline
\end{tabular}}
\caption{}
\end{subfigure}

\vspace*{0.3cm}
\caption{Computation of a TP set operation using the LIR:
(a) Lineage-Enhanced Temporal Relations
(b) Set-Intersection Result
(c) Normalizations
(d) Join on condition $\theta : r.F,T =s.F,T$}
\label{fig:NormExample}
\end{figure}

\begin{figure}[h]
\centering
\begin{subfigure}[b]{0.6\linewidth}
\centering
\scalebox{0.8} {
\begin{tabular}{ M{0.3cm} | M{0.7cm} | M{0.2cm} @{}m{0pt}@{}}
\multicolumn{3}{l}{\bf r}\\
\cline{1-3} 
$P$ &  $T$      & $\lambda$ & \\  \cline{1-3} %& $\lambda$
m    & {[2,10)} & {$r_1$} & \\ [0.1cm]
c     & {[4,7)}   & {$r_2$} & \\ [0.1cm]%& $A_3$ 
d     & {[1,3)}   & {$r_3$} & \\ [0.1cm]
\cline{1-3}
\end{tabular}}
\qquad
\scalebox{0.8} {
\begin{tabular}{ M{0.3cm} | M{0.7cm} | M{0.2cm} @{}m{0pt}@{}}
\multicolumn{3}{l}{\bf s }\\
\cline{1-3}   
$P$ &  $T$     & $\lambda$ & \\  \cline{1-3}  %& $\lambda$
m    & {[1,4)} & $s_1$  & \\ [0.1cm]
m    & {[6,8)} & $s_2$  &\\  [0.1cm]
c     & [4,5)    & $s_3$  & \\ [0.1cm]
c     & [7,9)    & $s_4$  & \\ [0.1cm] 
\cline{1-3}
\end{tabular}}
\caption{}
\end{subfigure}
\qquad
\begin{subfigure}[b]{0.3\linewidth}
\centering
\scalebox{0.8} {
\begin{tabular}{ M{0.3cm} | M{0.7cm} | M{0.75cm} @{}m{0pt}@{}}
\multicolumn{3}{l}{${\bf r} \cap^\kat{T} {\bf s}$}\\
\hline
$P$  & $T$    & $\lambda$         \\ \hline %& $\lambda$
m    & [2,4)  & $r_1 \cdot \ s_1$ \\ [0.1cm] 
m    & [6,8)  & $r_1 \cdot \ s_2$ \\ [0.1cm]
c     & [4,5)  & $r_2 \cdot \ s_3$ \\ [0.1cm] 
\hline
\end{tabular}}
\caption{}
\end{subfigure}
\vspace{0.2cm}

\begin{subfigure}[b]{0.58\linewidth}
\centering
\scalebox{0.8} {
\begin{tabular}{ M{0.3cm} | M{0.7cm} | M{0.3cm}  @{}m{0pt}@{}}
\multicolumn{4}{l}{$N(\mathbf{r},\mathbf{s})$}\\
\hline                                                       
$P$  & $T$     & $\lambda$ \\ \hline 
m    & [2,4)   & $r_1$ &\\ [0.1cm] 
m    & [4,6)   & $r_1$ &\\ [0.1cm]
m    & [6,8)   & $r_1$ &\\ [0.1cm]
m    & [8,10) & $r_1$ &\\ [0.1cm]
c     & [4,5)   & $r_2$ &\\ [0.1cm]
c     & [5,7)   & $r_2$ &\\ [0.1cm]
d     & [1,3)   & $r_3$ &\\ [0.1cm]
\hline
\end{tabular}}
\qquad
\scalebox{0.8} {
\begin{tabular}{ M{0.3cm} | M{0.7cm} | M{0.3cm} @{}m{0pt}@{}}
\multicolumn{4}{l}{$N(\mathbf{s},\mathbf{r})$}\\
\hline                                                       
$P$  & $T$   & $\mathtt{\lambda_s}$   \\ \hline 
m    & [1,2)  & $s_1$  &\\ [0.1cm]
m    & [2,4)  & $s_1$  &\\ [0.1cm] 
m    & [6,8)  & $s_2$  &\\ [0.1cm]
c     & [4,5)   & $s_3$  &\\ [0.1cm]
c     & [7,9)   & $s_3$  &\\ [0.1cm]
\hline
\end{tabular}}
\caption{}
\end{subfigure}
\qquad
\begin{subfigure}[b]{0.32\linewidth}
\centering
\scalebox{0.8} {
\begin{tabular}{ M{0.3cm} | M{0.7cm} | M{0.65cm} | M{0.65cm} @{}m{0pt}@{}}
\multicolumn{4}{l}{${\bf u} = \mathcal{N}(r;s) \ \Join\theta \ \mathcal{N}(s;r)$}\\
\hline
$P$  & $T$   & $r.\lambda$ & $s.\lambda$  \\ \hline %& $\lambda$
m    & [2,4)  & $r_1 $ & $s_1$ \\ [0.1cm] 
m    & [6,8)  & $r_1 $ & $s_2$ \\ [0.1cm]
c     & [4,5)  & $r_2$  & $s_3$ \\ [0.1cm] 
\hline
\end{tabular}}
\caption{}
\end{subfigure}

\vspace*{0.3cm}
\caption{Computation of a TP set operation using the LIR:
(a) Lineage-Enhanced Temporal Relations
(b) Set-Intersection Result
(c) Normalizations
(d) Join on condition $\theta : r.F,T =s.F,T$}
\label{fig:NormExample}
\end{figure}

{\color{red} I DO NOT AT ALL UNDERSTAND THE FOLLOWING. IS THIS NEEDED FOR CHANGE PRESERVATION?

\begin{lemma}
\label{lem:mainObservation}
Assume we have two temporal-probabilistic relations ${\bf r}$ and ${\bf s}$
both having schema ($F$, $\lambda$, $T$, $p$), and let $\mathtt{base}(\lambda)$ again denote set of the base tuples in a lineage expression $\lambda$. 
Then, all the facts included in either ${\bf r}\cap^\kat{Tp} {\bf s}$ or ${\bf r}-^\kat{Tp}{\bf s}$
are also included, during the same intervals, in the result of
${\bf r}\cup^\kat{Tp}{\bf s}$.

\vspace*{0.1cm}
% {\centering \noindent $\exists k \in {\bf k} \ (k.F=f \ \wedge
% \ k.T = T_\kat{F} \ \wedge \ \lambda_\kat{F} = \lambda_{fun}(\lambda_1,\lambda_2))$}
$\pi_{F,T,\mathtt{base}(\lambda)}({\bf r}\cup^\kat{Tp}{\bf s}) \supseteq
 \pi_{F,T,\mathtt{base}(\lambda)}({\bf r}-^\kat{Tp}{\bf s}) \supseteq
 \pi_{F,T,\mathtt{base}(\lambda)}({\bf r}\cap^\kat{Tp}{\bf s})$
\end{lemma}

\vspace*{0.1cm}
\begin{proof}
All the inclusion relationships in Lemma~\ref{lem:mainObservation} can
be similarly proven and thus, we will only prove $\pi_{F,T,\mathtt{base}
(\lambda)}({\bf r}\cup^\kat{Tp}{\bf s}) \supseteq \pi_{F,T,\mathtt{base}
(\lambda)} ({\bf r}\cap^\kat{Tp}{\bf s})$. For this inclusion to hold, all
tuples belonging in $\pi_{F,T,\mathtt{base}(\lambda)}({\bf r}\cap^\kat{Tp}
{\bf s})$ should also belong to $\pi_{F,T,\mathtt{base}(\lambda)}({\bf r}
\cup^\kat{Tp}{\bf s})$. We will assume that the statement $\exists
u \in \pi_{F,T,\mathtt{base}(\lambda)}({\bf r}\cap^\kat{Tp} {\bf s})\ (u \notin
\pi_{F,T,\mathtt{base}(\lambda)}({\bf r}\cup^\kat{Tp}{\bf s}))$ (1) and show
that this assumption leads to contradiction.

%Relations $\pi_{F,T,\mathtt{base}(\lambda)/\lambda_{set}}({\bf r}\cup^\kat{Tp}
%{\bf s})$ and $\pi_{F,T,\mathtt{base}(\lambda)/\lambda_{set}}({\bf r}\cap^
%\kat{TP}{\bf s})$ include all the tuples in ${\bf r}\cup^\kat{Tp}{\bf s}$
%and ${\bf r}\cup^\kat{Tp}{\bf s}$, after their lineage expressions have been
%replaced by the corresponding set of base tuples $L_b(\lambda)$. Consequently,
%each tuple in these relations

Assume tuple $u \in \pi_{F,T,\mathtt{base}(\lambda)/\lambda_{set}}({\bf r}
\cap^\kat{Tp}{\bf s})$. As all tuples in this relation, $u$ has been
derived from a tuple $u' \in \ {\bf r}\cap^\kat{Tp}{\bf s}$ with
$u'.F = u.F \wedge u'.T = u.T \wedge \mathtt{base}(u'.\lambda) =
u.\lambda_{set}$. Given that $u$ and $u'$ include the same fact and
interval, it holds that $r_u = r_{u'} \wedge s_u = s_{u'}$. Moreover,
since $u'$ belongs to the result of the TP set intersection, according
to Definition~\ref{def:TPsetOps}, it satisfies the corresponding interval
condition $i_c(u')$, the fact condition $r_{u'} \ne \mathtt{null} \wedge
s_{u'} \ne \mathtt{null}$ and the lineage condition $u.\lambda = r_{u'}.
\lambda \cdot s_{u'}.\lambda$. Consequently, $u$ also satisfies the
above interval and fact conditions. Also, by ignoring the logical
operators, the set of base tuples included in $u.\lambda_{set}$ is equal
to $\mathtt{base}(u'.\lambda) = \mathtt{base}(r_{u'}.\lambda \cdot s_{u'}.\lambda)
= L_b(r_{u}.\lambda)) \cup L_b(s_{u}.\lambda)$. 

According to our initial assumption (1), $u \notin \pi_{F,T,\mathtt{base}
(\lambda)/ \lambda_{set}}({\bf r}\cup^\kat{Tp}{\bf s})$. This means
that $u$ cannot have been derived from any tuple in ${\bf r}\cup^
\kat{TP}{\bf s}$. So, for all tuples $u''$ over the schema (F,T,
$\lambda$,p) with $u'.F = u.F \wedge u'.T = u.T \wedge \mathtt{base}
(u''.\lambda) = u.\lambda_{set}$, we conclude that $u'' \notin {\bf r}
\cup^\kat{Tp}{\bf s}$. Given that $u$ and $u'$ include the same fact
and interval, it holds that $r_u = r_{u''} \wedge s_u = s_{u''}$. Also,
given the interval and fact condition satisfied by $u$, it holds that $u''$
satisfies $i_c(u'')$ and $r_{u''} \ne \mathtt{null} \wedge s_{u''} \ne 
\mathtt{null}$. However, $u''\notin {\bf r}\cup^\kat{Tp}{\bf s}$. For this to
hold, based on Table~\ref{def:TPsetOps} and the interval and fact
conditions that $u''$ satisfies, $u''.\lambda \neq r_{u''}.\lambda \cdot
s_{u''}.\lambda$. As a consequence $\mathtt{base}(u''.\lambda) \neq
L_b(r_{u''}.\lambda)) \cup L_b(s_{u''}.\lambda) \neq L_b(r_{u}.
\lambda)) \cup L_b(s_{u}.\lambda)$. This contradicts our assumption
that $\mathtt{base}(u''.\lambda) = u.\lambda_{set}$ prooving that $u \notin
\pi_{F,T,\mathtt{base} (\lambda)/\lambda_{set}} ({\bf r}\cup^\kat{Tp}{\bf
s})$ is false, and thus $\pi_{F,T,\mathtt{base} (\lambda)}({\bf r}\cup^\kat{Tp}
{\bf s}) \supseteq \pi_{F,T,\mathtt{base}(\lambda)} ({\bf r}\cap^\kat{Tp}{\bf
s})$. 
\end{proof}}

\subsection{Test Abstract}
In this paper, we investigate the computation of temporal probabilistic (TP)
set-queries over duplicate-free relations. We adopt a data model whose query
semantics is consistent with sequenced semantics on the temporal dimension
and possible world semantics on the probabilistic one. We define TP
set-operations and we propose a novel lineage-aware sweeping window approach
for their computation that exploits the non-existence of duplicates. Our
lineage-aware window advancer LAWA produces candidate output intervals that can
be filtered at the time of their creation given the lineage expressions
of the tuples valid. Using a window sweeping technique it manages to cover
not only TP set-intersection, widely covered by sweepline approaches, but also
TP set-difference and union. LAWA computes TP set-operations in
$O(n \, \log n)$ time, thus improving over the best existing implementations
that require quadratic time under a sequenced temporal semantics.
A series of experiments on real and synthetic datasets show (a)
that LAWAs has predictable performance which only depends on the size
and not on the characteristics of the input intervals (such as the number
of distinct facts, overlap of intervals), and (b) that the LAWA
outperforms state-of-the-art approaches that implement temporal-probabilistic
IUE queries under a sequenced temporal semantics.

\subsection{Postgres Pipeline Extension}

\subsection{PostgreSQL Pipeline Extension}

This section describes how \emph{LIR$_{algo}$} primitive is
implemented in the kernel of the PostgreSQL database system via
the modification of each module of the pipeline. When a query is
submitted by the user in Postgres, the corresponding
query-string is initially processed by the \emph{ parser}. Based
on the grammar defined, the parser is able to identify all the
keywords involved and, based on them, build the so-called
\emph{raw parse-tree}. The first step in the incorporation of an
{\bf LIR} operator is an extension of the grammar with the
keyword {\bf LIR}, with syntax:

\begin{figure}[htbp!]  \centering \scalebox{0.95} {'(' table\_ref LIR
    table\_ref USING '(' name\_list ')' ')' alias\_clause}
\end{figure}

In the above statement, the two appearances of `table\_ref' correspond
to references in the two input relations. The `name\_list' is a list
including all the non-temporal attributes which are the same in both
relations. 

Given all the existing grammar rules, the parser creates an initial \emph{raw
parse-tree} which is afterwards passed on to the analyzer, that produces the
query tree. The analyzer adapts the parse tree by adding, in the proper positions,
new nodes which will guarantee the proper preprocessing (tagging, union, grouping,
sorting) of the relations involved in \emph{LIR$_{algo}$}. In Fig.~\ref{fig:Analyzer}, both
the raw parse-tree and the query tree are presented. 

\tikzstyle{bag} = [text width=5em, text centered]
\begin{figure}[htbp!]
\begin{subfigure} [b]{0.35\linewidth}
        \center
\scalebox{0.7}{
\begin{tikzpicture}[sloped]
\tikzstyle{level 1}=[level distance=1.5cm, sibling distance=2cm]
        \node[bag] {\large{\emph{LIR}}}
        child {node[bag, label=center:{{\bf  \large r}}] {}}
        child {node[bag, label=center:{{\bf  \large s}}] {}};
\end{tikzpicture}}
\caption{Raw Parse Tree}
\label{fig:initParseTree}
\end{subfigure}
\hfill
%%%%%%%%%%%%%%%%%%%%%%%%%%%%%%%%%%%%%%%%%%%%%%%%%%%%%%%%%%%%%%%%%%%%%%%%%%%%%
\begin{subfigure} [b]{0.48\linewidth}
        \center
\scalebox{0.7}{
\begin{tikzpicture}[sloped]
\tikzstyle{level 1}=[level distance=1cm, sibling distance=1.7cm]
\tikzstyle{level 2}=[level distance=1cm, sibling distance=1.5cm]
\tikzstyle{level 3}=[level distance=1cm, sibling distance=1cm]
\tikzstyle{level 3}=[level distance=1cm, sibling distance=2cm]
\node[bag] {\large{\emph{LIR}}}
   child{
       node[bag] {sorting$_{A,B,T_s,T_e}$}
       child{
         node[bag] {\large{${\bf \cup_{all}}$}}
           child {
              node[bag] {\large{${\bf \Pi_\kat{A,B,$T_s$,$T_e$,$\lambda$,0}}$}}
              %node[bag] {\large{${\bf \Pi_\kat{A,B,$T_s$,$T_e$,$T_s/P_1$,$\lambda/\lambda_s$}}$}}
              child {node[bag] {{\bf  \large r}}}
           }
           child {
              node[bag] {\large{${\bf \Pi_\kat{A,B,$T_s$,$T_e$,$\lambda$,1}}$}}
              %node[bag] {\large{${\bf \Pi_\kat{A,B,$T_s$,$T_e$,$T_e/P_1$,$\lambda/\lambda_s$}}$}}
              child {node[bag] {{\bf  \large s}}}
           }
       }
   };
\end{tikzpicture}}
\caption{Query Tree}
\label{fig:queryTree}
\end{subfigure}
\vspace{0.5cm}
\caption{Analyzer Modifications}
\label{fig:Analyzer}
\end{figure}

The modifications in the \emph{executor} involve the implementation of the
functions \emph{ExecInitLIR}, \emph{ExecLIR} and \emph{ExecEndLIR} for the
initialization, execution and finalisation of the evaluation of the result
of \emph{LIR$_{algo}$}. In the \emph{ExecInitLIR} function the structure needed for
the implementation of \emph{LIR$_{algo}$} is initialised while in the
\emph{ExecEndLIR} function, the algorithm is incorporated.
